# Supplementary material for: Non-unitary Trotter circuits for imaginary time evolution
Source: arXiv:2304.07917 source file (2023-10-29)
Supplement: Supplementary file 1 [file appendix1.tex]

\section{Circuit complexity} \label{sec:appendix}

\begin{table}[h!]
\centering
\begin{tabular}{ c|c|c|c|c|c|c|c }
 $n_{\text{sites}}$ & $n_p$ & width & $n_t$ & $g_{\text{trotter}}$ & $d_{\text{trotter}}$ & $g_{\text{lcu}}$ & $d_{\text{lcu}}$ \\
 \hline
 \multirow{3}{*}[\normalbaselineskip]{2} &
 \multirow{3}{*}[\normalbaselineskip]{3} &
 \multirow{3}{*}[\normalbaselineskip]{3} & 1 & 8 & 8 & 14 & 14 \\ 
 & & & 10 & 80 & 80 & 140 & 140 \\
 & & & 100 & 800 & 800 & 1400 & 1400 \\
 \multirow{3}{*}[\normalbaselineskip]{4} &
 \multirow{3}{*}[\normalbaselineskip]{7} &\multirow{3}{*}[\normalbaselineskip]{5} & 1 & 24 & 24 & 40 & 40 \\
 & & & 10 & 240 & 231 & 400 & 391 \\
 & & & 100 & 2400 & 2301 & 4000 & 3901 \\
 \multirow{3}{*}[\normalbaselineskip]{8} &
 \multirow{3}{*}[\normalbaselineskip]{15} &\multirow{3}{*}[\normalbaselineskip]{9} & 1 & 48 & 48 & 80 & 80 \\ 
 & & & 10 & 480 & 471 & 800 & 791 \\
 & & & 100 & 4800 & 4701 & 8000 & 7901 \\
 \multirow{3}{*}[\normalbaselineskip]{16} &
 \multirow{3}{*}[\normalbaselineskip]{31} &\multirow{3}{*}[\normalbaselineskip]{17} & 1 & 96 & 96 & 160 & 160 \\ 
 & & & 10 & 960 & 951 & 1600 & 1591 \\ 
 & & & 100 & 9600 & 9501 & 16000 & 15901 \\
 %\hline
\end{tabular}
\caption{Comparison of the circuit complexity of the TIM quantum circuits for the Trotterised PITE model and the LCU PITE model \cite{kosugi2021probabilistic} with no gate optimisation performed, decomposed into {\sc cnot} gates and single qubit gates, as the number of sites $n_{\text{sites}}$ and the number of time steps $n_t$ is changed. The number of Pauli strings comprising the Hamiltonian $n_p$ is also listed. The `width' denotes the number of qubits, $n_{\text{sites}}+1$. $g_{\text{trotter}}$/$d_{\text{trotter}}$ gives the {\sc cnot} gate count/depth for the Trotterised PITE circuits.
}
\label{tab:circuit_complexity_compare_lcu}
\end{table}

% \begin{table}[h!]
% \centering
% \begin{tabular}{ c|c|c|c|c|c }
%  $n_{\text{sites}}$ & $n_p$ & width & $n_t$ & $g$ & $d$ \\
%  \hline
%  \multirow{3}{*}[\normalbaselineskip]{2} & \multirow{3}{*}[\normalbaselineskip]{11} & \multirow{3}{*}[\normalbaselineskip]{5} & 1 & 40 & 38 \\ 
%  & & & 10 & 400 & 380 \\
%  & & & 100 & 4000 & 3800 \\
%  \multirow{3}{*}[\normalbaselineskip]{4} & \multirow{3}{*}[\normalbaselineskip]{25} &
%  \multirow{3}{*}[\normalbaselineskip]{9} & 1 & 104 & 94 \\ 
%  & & & 10 & 1040 & 913 \\
%  & & & 100 & 10400 & 9103 \\
%  \multirow{3}{*}[\normalbaselineskip]{8} & \multirow{3}{*}[\normalbaselineskip]{53} & \multirow{3}{*}[\normalbaselineskip]{17} & 1 & 232 & 206 \\ 
%  & & & 10 & 2320 & 2033 \\
%  & & & 100 & 23200 & 20303 \\
%  \multirow{3}{*}[\normalbaselineskip]{16} &
%  \multirow{3}{*}[\normalbaselineskip]{109} &
%  \multirow{3}{*}[\normalbaselineskip]{33} & 1 & 488 & 430 \\ 
%  & & & 10 & 4880 & 4273 \\
%  & & & 100 & 48800 & 42703 \\
%  %\hline
% \end{tabular}
% \caption{Circuit complexity of the 1D fermionic Hubbard model quantum circuits, decomposed into {\sc cnot} gates and single qubit gates, as the number of sites $n_{\text{sites}}$ and the number of time steps $n_t$ is changed. The number of Pauli strings comprising the Hamiltonian $n_p$ is also listed; one of these is always the tensor product of identity operators and is not simulated. The `width' denotes the number of qubits, $2 n_{\text{sites}} + 1$. $g$/$d$ gives the {\sc cnot} gate count/depth for the circuits.}
% \label{tab:circuit_complexity_optimise_false}
% \end{table}
\begin{table}[h!]
\centering
\begin{tabular}{ c|c|c|c|c|c|c|c }
 $n_{\text{sites}}$ & $n_p$ & width & $n_t$ & $g_{\text{trotter}}$ & $d_{\text{trotter}}$ & $g_{\text{lcu}}$ & $d_{\text{lcu}}$ \\
 \hline
 \multirow{3}{*}[\normalbaselineskip]{2} & \multirow{3}{*}[\normalbaselineskip]{11} & \multirow{3}{*}[\normalbaselineskip]{5} & 1 & 40 & 38 \\ 
 & & & 10 & 400 & 380 \\
 & & & 100 & 4000 & 3800 \\
 \multirow{3}{*}[\normalbaselineskip]{4} & \multirow{3}{*}[\normalbaselineskip]{25} &
 \multirow{3}{*}[\normalbaselineskip]{9} & 1 & 160 & 151 \\ 
 & & & 10 & 1600 & 1483 \\
 & & & 100 & 16000 & 14803 \\
 \multirow{3}{*}[\normalbaselineskip]{8} & \multirow{3}{*}[\normalbaselineskip]{53} & \multirow{3}{*}[\normalbaselineskip]{17} & 1 & 352 & 327 \\ 
 & & & 10 & 3520 & 3243 \\
 & & & 100 & 35200 & 32403 \\
 \multirow{3}{*}[\normalbaselineskip]{16} &
 \multirow{3}{*}[\normalbaselineskip]{109} &
 \multirow{3}{*}[\normalbaselineskip]{33} & 1 & 488 & 430 \\ 
 & & & 10 & 4880 & 4273 \\
 & & & 100 & 48800 & 42703 \\
 %\hline
\end{tabular}
\caption{Circuit complexity of the 1D fermionic Hubbard model quantum circuits, decomposed into {\sc cnot} gates and single qubit gates, as the number of sites $n_{\text{sites}}$ and the number of time steps $n_t$ is changed. The number of Pauli strings comprising the Hamiltonian $n_p$ is also listed; one of these is always the tensor product of identity operators and is not simulated. The `width' denotes the number of qubits, $2 n_{\text{sites}} + 1$. $g$/$d$ gives the {\sc cnot} gate count/depth for the circuits.}
\label{tab:circuit_complexity_optimise_false}
\end{table}

% \begin{figure}[h]
% \centering
% \begin{quantikz}
% \lstick{$\ket{0}$} &  \gate{R_y(\theta_0)} &\ctrl{1} \gategroup[4,steps=4,style={dashed,
% rounded corners,fill=blue!20, inner xsep=3.5pt},
% background,label style={label position=below,anchor=
% north,yshift=-0.2cm}]{{ x d}} & \qw & \qw &\gate{R_y(\theta_4)} &\qw  \\
% \lstick{$\ket{0}$} &  \gate{R_y(\theta_1)}  & \targ{}  & \ctrl{1} &\qw &\gate{R_y(\theta_5)} & \qw \\
% \lstick{$\ket{0}$} &  \gate{R_y(\theta_2)}  & \qw & \targ{} & \ctrl{1}  & \gate{R_y(\theta_6)} & \qw \\
% \lstick{$\ket{0}$} &  \gate{R_y(\theta_3)}  & \qw & \qw & \targ{} & \gate{R_y(\theta_7)} & \qw 
% \end{quantikz} \\
% \caption{The hardware efficient RY-ansatz for 4 qubits with d layers.}
% \label{fig:hea}
% \end{figure}
